# Supplementary material for: Stock Price Predictability and the Business Cycle via Machine Learning
Source: arXiv:2304.09937 source file (2023-04-06)
Supplement: Supplementary file 1 [file appendix-hyperparameters.tex]

\begin{singlespace}
\begin{xltabular}{\textwidth}{
|L{1}|L{0.6}|L{1.6}|L{0.7}|L{0.3}|L{0.5}|}  
    \caption{Best hyper-parameters from grid search} \\ \hline 
    \label{tab:best_hp} 
    Feature Set & Sub-periods & Training Set & Model & Lag, l & Width, w \\ \hline \hline
    \endfirsthead
    \caption[]{Best hyper-parameters from grid search} \\ \hline
    Feature Set & Sub-periods & Training Set & Model & Lag, l & Width, w \\ \hline \hline
    \endhead
    \hline
    Without VIX or RF & 01-10 & Non-Recession & BLSTM & 5 & 64 \\ \hline
    Without VIX or RF & 01-10 & Non-Recession & GRU & 5 & 64 \\ \hline
    Without VIX or RF & 01-10 & Non-Recession & LSTM & 5 & 32 \\ \hline
    Without VIX or RF & 01-10 & Non-Recession + Recession & BLSTM & 9 & 64 \\ \hline
    Without VIX or RF & 01-10 & Non-Recession + Recession & GRU & 7 & 64 \\ \hline
    Without VIX or RF & 01-10 & Non-Recession + Recession & LSTM & 5 & 32 \\ \hline
    Without VIX or RF & 07-20 & Non-Recession & BLSTM & 5 & 128 \\ \hline
    Without VIX or RF & 07-20 & Non-Recession & GRU & 5 & 128 \\ \hline
    Without VIX or RF & 07-20 & Non-Recession & LSTM & 7 & 32 \\ \hline
    Without VIX or RF & 07-20 & Non-Recession + Recession & BLSTM & 5 & 64 \\ \hline
    Without VIX or RF & 07-20 & Non-Recession + Recession & GRU & 5 & 64 \\ \hline
    Without VIX or RF & 07-20 & Non-Recession + Recession & LSTM & 9 & 64 \\ \hline
    Without VIX or RF & 69-76 & Non-Recession & BLSTM & 9 & 128 \\ \hline
    Without VIX or RF & 69-76 & Non-Recession & GRU & 5 & 128 \\ \hline
    Without VIX or RF & 69-76 & Non-Recession & LSTM & 7 & 64 \\ \hline
    Without VIX or RF & 69-76 & Non-Recession + Recession & BLSTM & 5 & 128 \\ \hline
    Without VIX or RF & 69-76 & Non-Recession + Recession & GRU & 5 & 128 \\ \hline
    Without VIX or RF & 69-76 & Non-Recession + Recession & LSTM & 5 & 32 \\ \hline
    Without VIX or RF & 73-80 & Non-Recession & BLSTM & 5 & 128 \\ \hline
    Without VIX or RF & 73-80 & Non-Recession & GRU & 5 & 128 \\ \hline
    Without VIX or RF & 73-80 & Non-Recession & LSTM & 7 & 128 \\ \hline
    Without VIX or RF & 73-80 & Non-Recession + Recession & BLSTM & 7 & 64 \\ \hline
    Without VIX or RF & 73-80 & Non-Recession + Recession & GRU & 5 & 128 \\ \hline
    Without VIX or RF & 73-80 & Non-Recession + Recession & LSTM & 5 & 128 \\ \hline
    Without VIX or RF & 80-83 & Non-Recession & BLSTM & 5 & 64 \\ \hline
    Without VIX or RF & 80-83 & Non-Recession & GRU & 5 & 64 \\ \hline
    Without VIX or RF & 80-83 & Non-Recession & LSTM & 5 & 32 \\ \hline
    Without VIX or RF & 80-83 & Non-Recession + Recession & BLSTM & 9 & 64 \\ \hline
    Without VIX or RF & 80-83 & Non-Recession + Recession & GRU & 7 & 128 \\ \hline
    Without VIX or RF & 80-83 & Non-Recession + Recession & LSTM & 5 & 128 \\ \hline
    Without VIX or RF & 81-91 & Non-Recession & BLSTM & 5 & 128 \\ \hline
    Without VIX or RF & 81-91 & Non-Recession & GRU & 5 & 128 \\ \hline
    Without VIX or RF & 81-91 & Non-Recession & LSTM & 7 & 64 \\ \hline
    Without VIX or RF & 81-91 & Non-Recession + Recession & BLSTM & 5 & 128 \\ \hline
    Without VIX or RF & 81-91 & Non-Recession + Recession & GRU & 7 & 64 \\ \hline
    Without VIX or RF & 81-91 & Non-Recession + Recession & LSTM & 5 & 64 \\ \hline
    Without VIX or RF & 90-02 & Non-Recession & BLSTM & 7 & 128 \\ \hline
    Without VIX or RF & 90-02 & Non-Recession & GRU & 5 & 128 \\ \hline
    Without VIX or RF & 90-02 & Non-Recession & LSTM & 5 & 128 \\ \hline
    Without VIX or RF & 90-02 & Non-Recession + Recession & BLSTM & 5 & 128 \\ \hline
    Without VIX or RF & 90-02 & Non-Recession + Recession & GRU & 5 & 128 \\ \hline
    Without VIX or RF & 90-02 & Non-Recession + Recession & LSTM & 5 & 128 \\ \hline
    With RF & 01-10 & Non-Recession & BLSTM & 5 & 128 \\ \hline
    With RF & 01-10 & Non-Recession & GRU & 7 & 64 \\ \hline
    With RF & 01-10 & Non-Recession & LSTM & 9 & 64 \\ \hline
    With RF & 01-10 & Non-Recession + Recession & BLSTM & 5 & 64 \\ \hline
    With RF & 01-10 & Non-Recession + Recession & GRU & 5 & 128 \\ \hline
    With RF & 01-10 & Non-Recession + Recession & LSTM & 7 & 64 \\ \hline
    With RF & 07-20 & Non-Recession & BLSTM & 5 & 64 \\ \hline
    With RF & 07-20 & Non-Recession & GRU & 7 & 64 \\ \hline
    With RF & 07-20 & Non-Recession & LSTM & 5 & 32 \\ \hline
    With RF & 07-20 & Non-Recession + Recession & BLSTM & 9 & 128 \\ \hline
    With RF & 07-20 & Non-Recession + Recession & GRU & 9 & 128 \\ \hline
    With RF & 07-20 & Non-Recession + Recession & LSTM & 9 & 128 \\ \hline
    With RF & 69-76 & Non-Recession & BLSTM & 5 & 64 \\ \hline
    With RF & 69-76 & Non-Recession & GRU & 5 & 128 \\ \hline
    With RF & 69-76 & Non-Recession & LSTM & 9 & 128 \\ \hline
    With RF & 69-76 & Non-Recession + Recession & BLSTM & 5 & 128 \\ \hline
    With RF & 69-76 & Non-Recession + Recession & GRU & 5 & 128 \\ \hline
    With RF & 69-76 & Non-Recession + Recession & LSTM & 5 & 32 \\ \hline
    With RF & 73-80 & Non-Recession & BLSTM & 5 & 128 \\ \hline
    With RF & 73-80 & Non-Recession & GRU & 5 & 128 \\ \hline
    With RF & 73-80 & Non-Recession & LSTM & 7 & 128 \\ \hline
    With RF & 73-80 & Non-Recession + Recession & BLSTM & 7 & 64 \\ \hline
    With RF & 73-80 & Non-Recession + Recession & GRU & 7 & 128 \\ \hline
    With RF & 73-80 & Non-Recession + Recession & LSTM & 5 & 128 \\ \hline
    With RF & 80-83 & Non-Recession & BLSTM & 5 & 64 \\ \hline
    With RF & 80-83 & Non-Recession & GRU & 5 & 64 \\ \hline
    With RF & 80-83 & Non-Recession & LSTM & 5 & 32 \\ \hline
    With RF & 80-83 & Non-Recession + Recession & BLSTM & 7 & 64 \\ \hline
    With RF & 80-83 & Non-Recession + Recession & GRU & 7 & 128 \\ \hline
    With RF & 80-83 & Non-Recession + Recession & LSTM & 5 & 128 \\ \hline
    With RF & 81-91 & Non-Recession & BLSTM & 5 & 128 \\ \hline
    With RF & 81-91 & Non-Recession & GRU & 5 & 128 \\ \hline
    With RF & 81-91 & Non-Recession & LSTM & 7 & 64 \\ \hline
    With RF & 81-91 & Non-Recession + Recession & BLSTM & 7 & 128 \\ \hline
    With RF & 81-91 & Non-Recession + Recession & GRU & 7 & 64 \\ \hline
    With RF & 81-91 & Non-Recession + Recession & LSTM & 5 & 64 \\ \hline
    With RF & 90-02 & Non-Recession & BLSTM & 5 & 128 \\ \hline
    With RF & 90-02 & Non-Recession & GRU & 5 & 128 \\ \hline
    With RF & 90-02 & Non-Recession & LSTM & 7 & 128 \\ \hline
    With RF & 90-02 & Non-Recession + Recession & BLSTM & 5 & 128 \\ \hline
    With RF & 90-02 & Non-Recession + Recession & GRU & 7 & 64 \\ \hline
    With RF & 90-02 & Non-Recession + Recession & LSTM & 5 & 128 \\ \hline
    With VIX & 01-10 & Non-Recession & BLSTM & 5 & 128 \\ \hline
    With VIX & 01-10 & Non-Recession & GRU & 5 & 64 \\ \hline
    With VIX & 01-10 & Non-Recession & LSTM & 5 & 64 \\ \hline
    With VIX & 01-10 & Non-Recession + Recession & BLSTM & 7 & 128 \\ \hline
    With VIX & 01-10 & Non-Recession + Recession & GRU & 7 & 64 \\ \hline
    With VIX & 01-10 & Non-Recession + Recession & LSTM & 5 & 128 \\ \hline
    With VIX & 07-20 & Non-Recession & BLSTM & 7 & 128 \\ \hline
    With VIX & 07-20 & Non-Recession & GRU & 5 & 128 \\ \hline
    With VIX & 07-20 & Non-Recession & LSTM & 5 & 64 \\ \hline
    With VIX & 07-20 & Non-Recession + Recession & BLSTM & 5 & 64 \\ \hline
    With VIX & 07-20 & Non-Recession + Recession & GRU & 5 & 128 \\ \hline
    With VIX & 07-20 & Non-Recession + Recession & LSTM & 7 & 64 \\ \hline
    With VIX & 90-02 & Non-Recession & BLSTM & 5 & 64 \\ \hline
    With VIX & 90-02 & Non-Recession & GRU & 5 & 64 \\ \hline
    With VIX & 90-02 & Non-Recession & LSTM & 7 & 128 \\ \hline
    With VIX & 90-02 & Non-Recession + Recession & BLSTM & 7 & 128 \\ \hline
    With VIX & 90-02 & Non-Recession + Recession & GRU & 5 & 64 \\ \hline
    With VIX & 90-02 & Non-Recession + Recession & LSTM & 5 & 128 \\ \hline
\end{xltabular}
\end{singlespace}
